# Supplementary material for: Near-perfect broadband quantum memory enabled by intelligent spinwave compaction
Source: arXiv:2505.02424 source file (2025-05-05)
Supplement: Supplementary file 1 [file supplementary_noiseless_Raman_memory.pdf]

# Supplementary Information: Near-perfect broadband quantum memory enabled by intelligent spinwave compaction

## I. SUPPLEMENTARY NOTE 1: MODEL OF RAMAN MEMORY WITH FWM

According to Ref. [1, 2], the equations of motion in a co-moving frame with dimensionless time $t = \gamma\tilde{t}$ and coordinate $z = \tilde{z}/L$ ($\gamma$ is the decay rate of excited state and $L$ is the length of atomic ensemble) for the signal field, $\hat{E}_s$, and the anti-Stokes field, $\hat{E}_a$, and spin-wave excitation $\hat{S} = \sqrt{N}\hat{\sigma}_{gm}(z,t)$ (where $\hat{\sigma}_{gm}(z,t)$ are slowly varying collective atomic operators and $N$ is the number density of atoms in the ensemble) are given by

$$\frac{\partial}{\partial z}\hat{E}_s = -\sqrt{d}\frac{\Omega}{\Delta_s}\hat{S} - i\frac{d}{\Delta_s}\hat{E}_s, \tag{1}$$

$$\frac{\partial}{\partial z}\hat{E}_a^\dagger = -\sqrt{d}\frac{\Omega^*}{\Delta_a}\hat{S} + i\frac{d}{\Delta_a + \Delta_{hf}}\hat{E}_a^\dagger, \tag{2}$$

$$\frac{\partial}{\partial t}\hat{S} = \sqrt{d}\left(\frac{\Omega^*}{\Delta_s}\hat{E}_s - \frac{\Omega}{\Delta_a}\hat{E}_a^\dagger\right) - i\left(\frac{1}{\Delta_s} - \frac{1}{\Delta_a}\right)|\Omega|^2\hat{S}, \tag{3}$$

where $d = \kappa^2 NL/(\gamma c)$ is the optical depth of the ensemble with coupling coefficient $\kappa$ of light and atoms. The detuning of anti-Stokes $\Delta_a = \Delta_s + \Delta_{hf}$ where $\Delta_s$ is the detuning of the signal and $\Delta_{hf}$ is the energy difference between $|m\rangle$ and $|g\rangle$. All of the detunings and the Rabi frequency in dimensionless equations have been nomalized to the decay rate of the excited state $|e\rangle$. Due to the large detuning $\Delta_s \gg 1$, we have neglect the decay term and the incoming noise described by the Langevin noise. Here we assume that all atoms are initially pumped into the ground state and the population remains nearly unchanged due to the excitations are small compared to the total atoms. The operators obey the commutation relations

$$[\hat{S}(z,t), \hat{S}^\dagger(z',t')] = \delta(z-z')\delta(t-t'), \tag{4}$$

$$[\hat{E}_s(z,t), \hat{E}_s^\dagger(z',t')] = [\hat{E}_a(z,t), \hat{E}_a^\dagger(z',t')] = \delta(z-z')\delta(t-t'). \tag{5}$$

To simplify the equations, we define a "scaled time" $p(t) = \int_{-\infty}^{t}|\Omega(t')|^2dt'/\int_{-\infty}^{\infty}|\Omega(t')|^2dt'$, the "normalized" signal, anti-Stokes field and the corresponding spin wave as

$$\hat{a}_s(\tilde{z},p) = \Omega^*\hat{E}_s\frac{dt}{dp}e^{i\left(\frac{1}{\Delta_s}-\frac{1}{\Delta_a}\right)p + i\frac{d}{\Delta_s}z}, \tag{6}$$

$$\hat{a}_a^\dagger(\tilde{z},p) = \Omega\hat{E}_a^\dagger\frac{dt}{dp}e^{i\left(\frac{1}{\Delta_s}-\frac{1}{\Delta_a}\right)p - i\frac{d}{\Delta_a+\Delta_{hf}}z}, \tag{7}$$

$$\hat{s}(\tilde{z},p) = \hat{S}e^{i\left(\frac{1}{\Delta_s}-\frac{1}{\Delta_a}\right)p + i\frac{d}{\Delta_s}z}. \tag{8}$$

Here $\frac{dt}{dp}$ is the Jacob matrix for the coordinate transform. The corresponding commutation relations of these new operators are

$$[\hat{s}(z,p), \hat{s}^\dagger(z',p')] = \delta(z-z')\delta(p-p'), \tag{9}$$

$$[\hat{a}_s(z,p), \hat{a}_s^\dagger(z,p')] = [\hat{a}_a(z,p), \hat{a}_a^\dagger(z',p')] = \delta(z-z')\delta(p-p'), \tag{10}$$

Then the normalized equations are

$$\frac{\partial}{\partial z}\hat{a}_s = -g_s\hat{s}, \tag{11}$$

$$\frac{\partial}{\partial z}\hat{a}_a^\dagger = -g_a\hat{s}e^{-i\Delta kz}, \tag{12}$$

$$\frac{\partial}{\partial p}\hat{s} = g_s\hat{a}_s - g_a\hat{a}_a^\dagger e^{i\Delta kz}, \tag{13}$$

where $g_s = \frac{\sqrt{d}}{\Delta_s}(g_a = \frac{\sqrt{d}}{\Delta_a})$ is the effective coupling of between signal (anti-Stokes). $\Delta k = \frac{d}{\Delta_s} + \frac{d}{\Delta_a+\Delta_{hf}}$ is the wave vector mismatch of the two lights.

From the equations inherent twin generation feature of FWM process, there is an invariance relation between the anti-Stokes and signal in the equations which can be expressed as

$$g_a\frac{\partial}{\partial z}\hat{a}_s = g_s\frac{\partial}{\partial z}\hat{a}_a^\dagger e^{i\Delta kz}. \tag{14}$$

Then we can define a bright excitation of light $\hat{b} = (g_s\hat{a}_s - g_a\hat{a}_a^\dagger e^{i\Delta k\tilde{z}})/g$ with the effective coupling coefficient $g = \sqrt{g_s^2 - g_a^2}$ between $\hat{b}$ and $\hat{s}$. The equation can be simplified as

$$\frac{\partial}{\partial z}\hat{b} = -g\hat{s} + i\frac{\Delta k g_a}{g}\hat{a}_a^\dagger e^{i\Delta kz}, \tag{15}$$

$$\frac{\partial}{\partial p}\hat{s} = g\hat{b}. \tag{16}$$

When considering a near-perfect memory process, the small coupling of the anti-Stokes which gives $\frac{\Delta k g_a}{g}\hat{a}_a^\dagger e^{i\Delta kz} \ll 1$ and the equations become

$$\frac{\partial}{\partial z}\hat{b} = -g\hat{s}, \tag{17}$$

$$\frac{\partial}{\partial p}\hat{s} = g\hat{b}. \tag{18}$$

The equations can be solved by using Laplace transform in $z$ [3] as

$$\hat{s} = \frac{\partial}{\partial z}[\int_0^z J_0(2g\sqrt{z'p})\hat{s}_{in}(z-z')dz'] + g\int_0^p J_0(2g\sqrt{p'z})\hat{b}_{in}(p-p')dp' \tag{19}$$

$$\hat{b} = \frac{\partial}{\partial p}[\int_0^p J_0(2g\sqrt{p'z})\hat{b}_{in}(p-p')dp'] + g\int_0^z J_0(2g\sqrt{z'p})\hat{s}_{in}(z-z')dz' \tag{20}$$

As we can see, the spin and light fields are coupled by the zero-order of the first kind Bessel function $J_0$. The generation function of the Raman process is determined by the coupling equations of $\hat{b}$ and $\hat{s}$. By defining an evolution parameter $r = \sqrt{zp}$ and $\theta = tan^{-1}\sqrt{z/p}$ and separate the variables as $\hat{s} = \hat{\Phi}_s(r)\hat{\Psi}_s(\theta)$ and $\hat{b} = \hat{\Phi}_b(r)\hat{\Psi}_b(\theta)$, we can rewrite the equations as

$$\left[r\frac{\partial}{\partial r}\left(r\frac{\partial}{\partial r}\right)\right]\hat{\Phi}_i(r) + \left(r^2-\mu\right)\hat{\Phi}_i(r) = 0 \tag{21}$$

$$\left[\sin 2\theta\frac{\partial}{\partial\theta}\left(\sin 2\theta\frac{\partial}{\partial\theta}\right)\right]\hat{\Psi}_i(\theta) + 4\mu\hat{\Psi}_i(\theta) = 0, \tag{22}$$

where $i$ represents $b/s$. The first equation is a Bessel equation, and the second equation is a Euler equation. This is why the generation function is a Bessel function.

## II. SUPPLEMENTARY NOTE 2: HANKEL TRANSFORM MAPPING

By defining the modified Bessel function as $j_m(x,y) = \sqrt{y/x}^m J_m(2g\sqrt{xy})$[4], we can define a modified Hankel transform as$\hat{\mathcal{H}}_m\{f(x)\}(y) = g\int_0^x j_m[(x-x'),y]f(x')dx'$ which can rewrite the solutions as Eq. 3 in maintext. When considering the coversion between spin wave and light excitations, we have

$$\hat{s}(z,p) = \hat{\mathcal{H}}_0\{\hat{b}_{in}(p')\} + \hat{s}_{in}(z) - \hat{\mathcal{H}}_1\{\hat{s}_{in}(z')\}, \tag{23}$$

$$\hat{b}(z,p) = \hat{\mathcal{H}}_0\{\hat{s}_{in}(z')\} + \hat{b}_{in}(p) - \hat{\mathcal{H}}_1\{\hat{b}_{in}(p')\}. \tag{24}$$

When applying the modified Hankel transform $\hat{\varsigma}(k_z,p) = g\int_0^\infty J_0(2g\sqrt{k_z z})\hat{s}(z,p)dz$ and $\hat{\beta}(z,k_p) = g\int_0^\infty J_0(2g\sqrt{k_p p})\hat{b}(z,p)dp$, we can obtain the Hankel spectrum of $\hat{b}$ and $\hat{s}$ as

$$\hat{\varsigma}(k_z,p) = \begin{cases} \frac{1}{g}\hat{b}_{in}(p-k_z) & 0 \le k_z \le p \\ \hat{\varsigma}_{in}(k_z-p) & k_z > p \end{cases}, \tag{25}$$

$$\hat{\beta}(z,k_p) = \begin{cases} \frac{1}{g}\hat{s}_{in}(z-k_p) & 0 \le k_p \le z \\ \hat{\beta}_{in}(k_p-z) & k_p > z \end{cases}, \tag{26}$$

The spectrum of the generated spin wave $\hat{\varsigma}$ is composed of two parts, one is from the initial spin wave $\hat{\varsigma}_{in}$ but shifted away by $p$ and the other one is from the input signal $\hat{b}_{in}$ which is backward resized to $k_z$. Similarly, the spectrum of the generated spin wave $\hat{\beta}$ is also composed of two parts, one is from the input signal $\hat{\beta}_{in}$ but shifted away by $z$ and the other one is from the initial spin wave $\hat{s}_{in}$ which is backward resized to $k_p$.

For the case with infinite control power or infinite length of ensemble, the transformation between spin wave and optical excitation only governed by

$$\hat{\varsigma}(k_z,p) = \frac{1}{g}\hat{b}_{in}(p-k_z), \tag{27}$$

$$\hat{\beta}(z,k_p) = \frac{1}{g}\hat{s}_{in}(z-k_p). \tag{28}$$

With an inverted Hankel transform, these expressions are equivalent to

$$\hat{s}(z,p) = \hat{\mathcal{H}}_0\{\hat{b}_{in}(p')\}, \tag{29}$$

$$\hat{b}(z,p) = \hat{\mathcal{H}}_0\{\hat{s}_{in}(z')\}. \tag{30}$$

Due to the convolution properties of the transform, the optimal input excitation of light in write process should be temporally reversed against the readout one as

$$\hat{b}_{in}(1-p) = \hat{b}_r(p) \tag{31}$$

This can be easily proved by substituting Eq. 29 into Eq. 30. Similarly, we can prove that the optimal initial spin wave of the read process should be spatially reversed against the generated one.

$$\hat{s}_{in}(1-z) = \hat{s}_w(z) \tag{32}$$

According to the Hankel transform relation, the optimal spectrum of input light excitation should be compact to ensure a compact spinwave distribution. The optimal light excitation can be obtained by manipulating the waveform of the write pulse. While the optimal spin wave for read process is achieved by the optimal write process and a backward retrieval light. As a result, the Raman process becomes a time reversal process for the signal and the spatial reversal process for the spin wave.

## III. SUPPLEMENTARY NOTE 3: THE NOISE INDUCED BY FWM PROCESS

In write process, the invariance relation of FWM process gives

$$\hat{a}^{\dagger}_{a,l} - \hat{a}^{\dagger}_{a,in} = \xi \int_0^z e^{-i\Delta kz} \partial_z \hat{a}_s dz, \tag{33}$$

$$= \xi \int_0^z e^{-i\Delta kz} \frac{g}{g_s} \partial_z \hat{b} dz + \xi^2 \int_0^z e^{-i\Delta kz} \partial_z (\hat{a}^{\dagger}_a e^{i\Delta kz}) dz. \tag{34}$$

where $\hat{a}_{s,l}$ is the leaked signal and $\hat{a}^{\dagger}_{a,l}$ is the generated anti-Stokes and $\xi = g_a/g_s$. A $g_a \ll g_s$ in our experiment, resulting $g \approx g_s$ and $\xi^2 \ll 1$. Then the generated anti-Stokes can be reduced to

$$\hat{a}^{\dagger}_{a,l} \approx \xi \int_0^z e^{-i\Delta kz} \partial_z \hat{b} dz + \hat{a}^{\dagger}_{a,in}. \tag{35}$$

$$\approx -g_a \int_0^z e^{-i\Delta kz} \hat{s} dz + \hat{a}^{\dagger}_{a,in}. \tag{36}$$

Therefore,

$$\hat{E}^{\dagger}_{a,out} \propto -g_a \int_0^L e^{-i\Delta kz} \hat{s} dz. \tag{37}$$

Considering a vacuum input of anti-Stokes, we neglect the term $\hat{a}^{\dagger}_{a,in}$ since it is small. The first term arises from the distribution of generated spinwave within the ensemble. The longer the spin wave, the more intense the anti-Stokes. Therefore, a compact spin wave greatly shortens the distribution of spin wave, which suppresses the propagation effect of FWM amplification.

## IV. SUPPLEMENTARY NOTE 4: THE DE ALGORITHM

Constrained by the limited bandwidth of the AOM, we use a near Gaussian-shaped write pulse in our demonstration which also achieves a near-perfect quantum memory. In this experiment, the DE algorithm is employed to optimize the pulse center and duration of a Gaussian-shaped write pulse. The algorithm takes the memory efficiency recorded by the oscilloscope as input and searches in a set of pulse center and duration for the best waveforms. The potential waveforms are then synthesized by an arbitrary signal generator. During optimizing, the algorithm initially selects the waveform with high efficiency from a set of random waveforms $\{\Omega_1^0(t), ..., \Omega_i^0(t)\}$. Subsequently, the algorithm generates a series of new waveforms $\{\Omega_1^1(t), ..., \Omega_i^1(t)\}$ by adding a differential waveform of two randomly chosen waveforms within the same generation to the selected waveform. The newly identified high-efficiency waveform may then be selected again for the next generation of waveforms $\{\Omega_1^2(t), ..., \Omega_i^2(t)\}$. This process of selection and generation continues iteratively until the efficiency improvement plateaus or a specified upper limit of generations is reached, signaling the completion of the optimization. Finally, the optimal waveform of the write pulse is determined based on the one yielding the highest efficiency.

---

[1] S. E. Thomas, T. M. Hird, J. H. D. Munns, B. Brecht, D. J. Saunders, J. Nunn, I. A. Walmsley, and P. M. Ledingham, Raman quantum memory with built-in suppression of four-wave-mixing noise, Physical Review A 100, 033801 (2019).

[2] Alexey V. Gorshkov, Axel Andre, Mikhail D. Lukin, and Anders S. Sorensen. Photon storage in Λ-type optically dense atomic media. ii. free-space model. Physical Review A, 76(3):033805 (2007).
[3] M. G. Raymer and J. Mostowski, Stimulated Raman scattering: Unified treatment of spontaneous initiation and spatial propagation, Physical Review A, 24, 1980 (1981).
[4] Ben Hamadi, N., Hafirassou, Z. & Herch, H. Uncertainty principles for the Hankel–Stockwell transform. Journal of Pseudo-Differential Operators and Applications, 11, 543–564 (2020).
